# Supplementary material for: Rich Ground State Chemical Ordering in Nanoparticles: Exact Solution of a Model for Ag-Au Clusters
Source: arXiv:1712.07427 ancillary file (2018-06-13)
Supplement: Supplementary file 1 [file supplementary.pdf]

# Rich Ground State Chemical Ordering in Nanoparticles: Exact Solution of a Model for Ag-Au Clusters. Supplementary Information.

Peter Mahler Larsen, Karsten Wedel Jacobsen, and Jakob Schiøtz*

*Center for Atomic-scale Materials Design (CAMD), Department of Physics, Technical University of Denmark, 2800 Kongens Lyngby, Denmark*

(Dated: March 28, 2018)

## S1. DRIVING FORCES OF STRUCTURAL EVOLUTION

As described in the results section in the manuscript, the driving force of the structural evolution is a trade-off between the energetic differences between site types and the preference for Ag and Au to form heteroatomic bonds. The effect of the former is quantified in Fig. 4. The latter is quantified here, using a CE model which contains clusters for nearest neighbour bonds only. By solving the resulting MIP model, we can determine the maximum number of heteroatomic bonds permitted by the nanoparticle site geometry.

Figure S1 compares this with the number of heteroatomic bonds in the ground state AgAu nanoparticles at every concentration. At low and high concentrations of Au, the preference for low-energy sites can be accommodated without any reduction in the number of heteroatomic bonds. The trade-off is visible in the central concentration region, where the number of heteroatomic bonds significantly lower than the maximum. At the same time, the preference for heteroatomic bonding produces a more complex configuration than that which would result if the site energetics were the only factor.

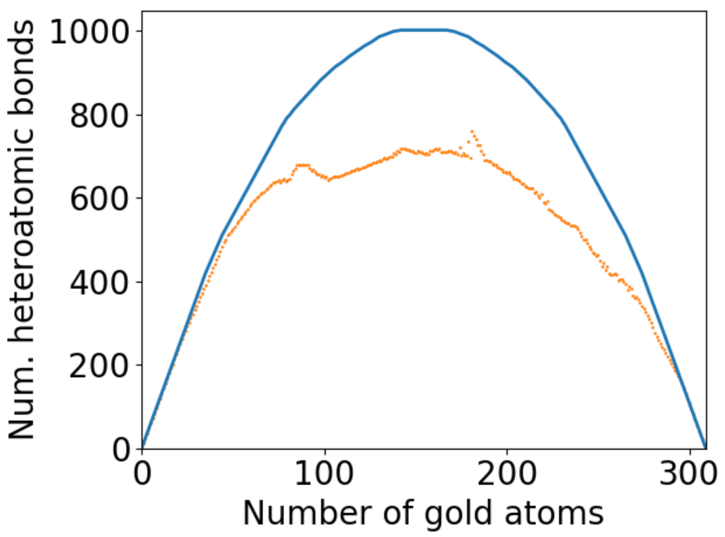


FIG. S1. Number of heteroatomic nearest-neighbour bonds in the AgAu ground state nanoparticles (red) and the maximum number of heteroatomic nearest-neighbour bonds permitted by the geometry of the nanoparticle (blue).

## S2. EXCITED STATES

The stability of the nanoparticle ground states can be understood in terms of the driving forces described above. Figure S2 shows the ground state and first excited state for three stoichiometries. The difference in formation energy is large for $Ag_{296}Au_{13}$ and $Ag_{296}Au_{13}$. Here, the ground state configurations exhibit perfect icosahedral symmetry and full Au occupation of certain site types: subsurface corners and the central atom in $Ag_{296}Au_{13}$, and the 1$^{st}$ and 3$^{rd}$ shells in $Ag_{296}Au_{13}$. An excited state therefore necessitates placement of an Au atom at a higher energy site.

The excited state of $Ag_{162}Au_{147}$ incurs a small energetic penalty relative to the ground state. The site types occupied by Ag and Au atoms are identical, and the number of heteroatomic-nearest neighbour bonds is unchanged. The ground state is effectively degenerate, as there exist multiple configurations of similar energy which differ only in their longer range interactions. In general, a ground state is degenerate if there exist other configurations with the same site type occupancy and number of heteroatomic bonds; all excited states which meet this condition have excitation energies below 2 meV.

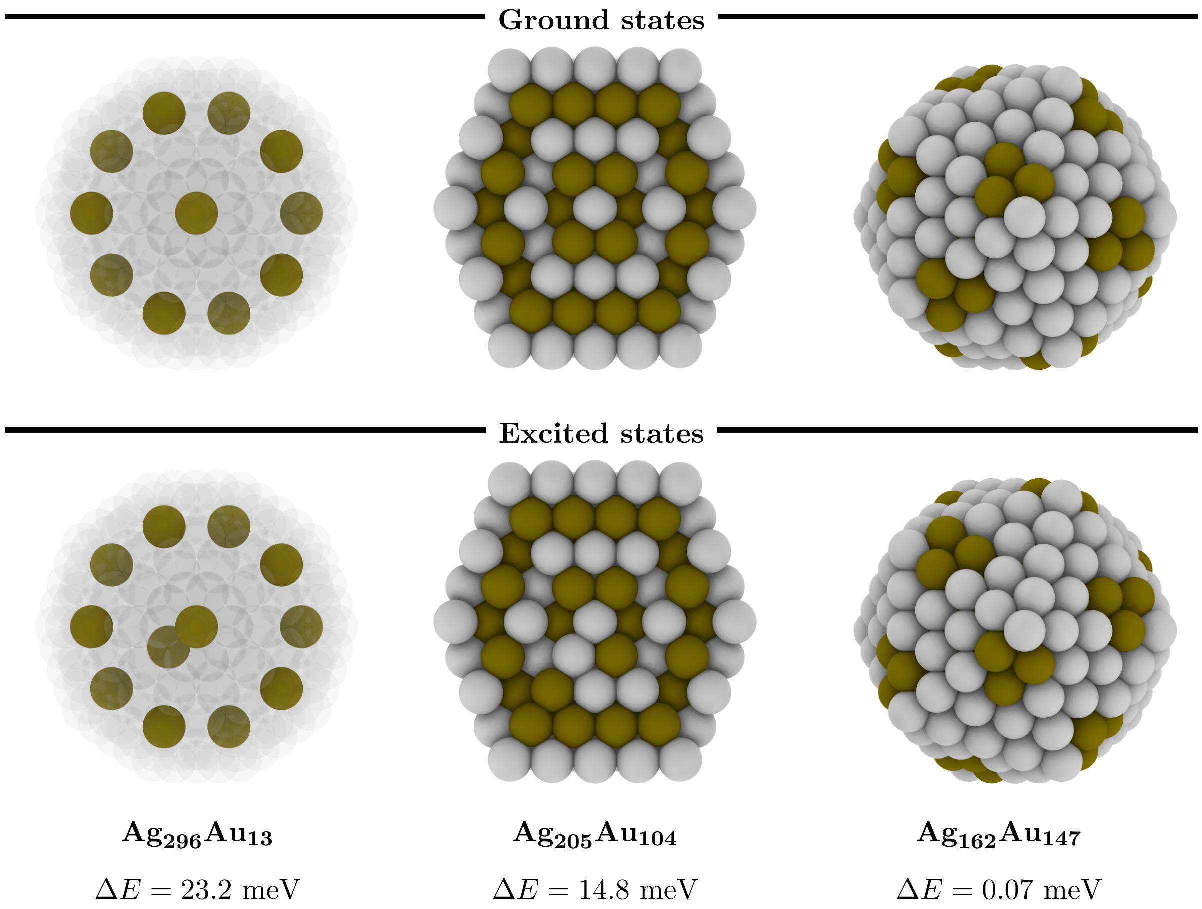


FIG. S2. Ground states (top) and the first excited states (bottom) for three different stoichiometries, and the corresponding excitation energies.

## S3. NOTES ON CLUSTER EXPANSION MODEL

The current best practice for cluster and ECI selection is to use compressive sensing [1, 2], though this is motivated by the need to construct a sparse model from limited data. The use of a semi-empirical potential, however, permits the sampling of a vast number of configurations, which in turn allows for a simple calculation of the ECIs. We have sampled 75,000 chemical ordering configurations, using a mixture of random sampling and stochastic local search in order to include configurations with both high and low energies; sampling a wider range of energies in this way has been shown to improve the generalization of a CE model [3]. The energy of each configuration has been minimized using gradient descent to allow local relaxations without changing the overall structure of the nanoparticle. The calculations were performed using the Atomic Simulation Environment, ASE [4, 5].

To select clusters, we generate all 1, 2, and 3-body clusters with a maximum site-site distance of three, where the inter-site distance is given by the number of nearest-neighbour 'hops' between the sites. From the resulting 2699 clusters, we identify relevant clusters with iterated local search [6], producing a smaller CE model with 60 1-body, 2-body and 3-body clusters, which contain a total of 4077 cluster instances. The resulting CE model is robust; when measured against a set of $20,000$ configurations not used in the fitting process, the CE model has a root-mean-square error (RMSE) of 0.060 meV/atom, which increases to 0.195 meV/atom when measured against the out-of-sample ground-state structures found using the MIP model.

All MIP models were solved using the Gurobi 7.5 optimization library [7].

* schiotz@fysik.dtu.dk

[1] L. J. Nelson, G. L. W. Hart, F. Zhou, and V. Ozolins, Phys. Rev. B **87**, 035125 (2013).

[2] L. J. Nelson, V. Ozolins, C. S. Reese, F. Zhou, and G. L. W. Hart, Phys. Rev. B **88**, 155105 (2013).

[3] A. Seko, Y. Koyama, and I. Tanaka, Phys. Rev. B **80**, 165122 (2009).

[4] S. R. Bahn and K. W. Jacobsen, Comput. Sci. Eng. **4**, 56 (2002).

[5] A. H. Larsen, J. J. Mortensen, J. Blomqvist, I. E. Castelli, R. Christensen, M. Dułak, J. Friis, M. N. Groves, B. Hammer, C. Hargus, E. D. Hermes, P. C. Jennings, P. B. Jensen, J. Kermode, J. R. Kitchin, E. L. Kolsbjerg, J. Kubal, K. Kaasbjerg, S. Lysgaard, J. B. Maronsson, T. Maxson, T. Olsen, L. Pastewka, A. Peterson, C. Rostgaard, J. Schiøtz, O. Schütt, M. Strange, K. S. Thygesen, T. Vegge, L. Vilhelmsen, M. Walter, Z. Zeng, and K. W. Jacobsen, J Phys Condens Matter **29**, 273002 (2017).

[6] H. R. Lourenço, O. C. Martin, and T. Stützle, in *Handbook of metaheuristics* (Springer, 2010) pp. 363–397.

[7] Gurobi Optimization, Inc., "Gurobi optimizer reference manual," `http://www.gurobi.com` (2016).
